# Supplementary material for: Machine- and deep-learning-driven angular momentum inference from BHEX observations of the $n=1$ photon ring
Source: arXiv:2411.01060 source file (2024-11-01)
Supplement: Supplementary file 1 [file appendix.tex]

\section{Helpful thing 1}
